# Supplementary material for: Latent Variable Method Demonstrator -- Software for Understanding Multivariate Data Analytics Algorithms
Source: arXiv:2205.08132 source file (2022-09-26)
Supplement: Supplementary file 1 [file AAppendix.tex]

\section{\acrshort{lavade} Detailed Results}
\label{sec:aappend}

\paragraph*{Default Case}

The following figures show detailed results of the default case described in section \ref{sec:CaseStudies}.

\begin{figure}[H]
    \centering
    \includegraphics[scale=0.125]{Figures/DefaultCase/Tool/DC_PLS_1_4.png}
    \caption{\acrshort{pls}, Obeserved $R^2$ on Test Data between 0.49 and 1.0, depending on $\mathbf{X}$}
    \label{fig:DC_pls}
\end{figure}

\begin{figure}[H]
    \centering
    \includegraphics[scale=0.125]{Figures/DefaultCase/Tool/DC_PCR_1_0.png}
    \caption{\acrshort{pcr}}
    \label{fig:DC_pcr}
\end{figure}

\begin{figure}[H]
    \centering
    \includegraphics[scale=0.125]{Figures/DefaultCase/Tool/DC_LASSO.png}
    \caption{LASSO}
    \label{fig:DC_lasso}
\end{figure}

\begin{figure}[H]
    \centering
    \includegraphics[scale=0.125]{Figures/DefaultCase/Tool/DC_RR.png}
    \caption{\acrshort{rr}}
    \label{fig:DC_RR}
\end{figure}

\begin{figure}[H]
    \centering
    \includegraphics[scale=0.125]{Figures/DefaultCase/Tool/DC_EN.png}
    \caption{\acrshort{en}}
    \label{fig:DC_EN}
\end{figure}

\paragraph*{Default Standardized Case}

The following figures show detailed results of the default standardized case described in section \ref{sec:CaseStudies}.

\begin{figure}[H]
    \centering
    \includegraphics[scale=0.125]{Figures/DefaultSCase/Tool/DSC_LASSO.png}
    \caption{\acrshort{lasso}}
    \label{fig:DSC_LASSO}
\end{figure}

\begin{figure}[H]
    \centering
    \includegraphics[scale=0.125]{Figures/DefaultSCase/Tool/DSC_PCR_1_0.png}
    \caption{\acrshort{pcr}}
    \label{fig:DSC_PCR}
\end{figure}

\begin{figure}[H]
    \centering
    \includegraphics[scale=0.125]{Figures/DefaultSCase/Tool/DSC_PLS_1_0.png}
    \caption{\acrshort{pls}}
    \label{fig:DSC_PLS}
\end{figure}

\paragraph*{Noisy Case}

The following figures show detailed results of the noisy described in section \ref{sec:CaseStudies}.

\begin{figure}[H]
    \centering
    \includegraphics[scale=0.125]{Figures/NoisyCase/Tool/NC_LASSO.png}
    \caption{\acrshort{lasso}}
    \label{fig:NC_LASSO}
\end{figure}

\begin{figure}[H]
    \centering
    \includegraphics[scale=0.125]{Figures/NoisyCase/Tool/NC_PLS_1.png}
    \caption{\acrshort{pls} 1 component}
    \label{fig:NC_PLS1}
\end{figure}

\begin{figure}[H]
    \centering
    \includegraphics[scale=0.125]{Figures/NoisyCase/Tool/NC_PLS_4.png}
    \caption{\acrshort{pls} 4 components}
    \label{fig:NC_PLS4}
\end{figure}

\begin{figure}[H]
    \centering
    \includegraphics[scale=0.125]{Figures/NoisyCase/Tool/NC_PLS_20.png}
    \caption{\acrshort{pls} 20 components}
    \label{fig:NC_PLS20}
\end{figure}

\begin{figure}[H]
    \centering
    \includegraphics[scale=0.125]{Figures/NoisyCase/Tool/NC_RR.png}
    \caption{\acrshort{rr} single run}
    \label{fig:NC_RR}
\end{figure}

\begin{figure}[H]
    \centering
    \includegraphics[scale=0.125]{Figures/NoisyCase/Tool/NC_RR_Mult.png}
    \caption{\acrshort{rr} Multiple Runs}
    \label{fig:NC_RR_multiple}
\end{figure}
